# Supplementary material for: Numerical Study of Geometric Multigrid Methods on CPU--GPU Heterogeneous Computers
Source: arXiv:1208.4247 source file (2013-01-11)
Supplement: Supplementary file 1 [file appendix.tex]

%!TEX root = main.tex

\section{Appendix}\label{sec:append}

\subsection{Implementation Details}

\begin{table}[H] %[htbp]
  \centering
  \small
  \caption{Experiment Environment}\label{CentOS6.2}
  \begin{tabular}{cl} \hline
          CPU       & AMD FX(tm)-8150 \\ \hline
          CPU Clock  & 3.6 GHz $\times 8$\\ \hline
          Host Memory & 16GB \\ \hline
          GPU       & Nvidia Geforce Gtx 480  \\ \hline
           CUDA Capability & 2.0 \\ \hline
          GPU Clock & 1.4 GHz $\times 15 \times 32$ cores \\ \hline
          Device Memory & 1.5GB \\ \hline
           OS       & CentOS 6.2 \\ \hline
          CUDA Driver & 4.1 \\ \hline
      Host Compiler & gcc 4.4.6 \\ \hline
    Device Compiler & nvcc 4.1 \\ \hline
  \end{tabular}
  \small
\end{table}

%\begin{table}[H]
%{\centering
%   \caption{ Theoretical peak capabilities of the device used in tests }\label{Theoretical_peak_gtx480}
%   \vskip 0.2cm
%    \begin{tabular}{lr} \hline
%      &Nvidia Geforce Gtx 480   \\ \hline
%   single prec. perform. [TFLOPS]   & 1.30    \\ %\hline
%   double prec. perform. [GFLOPS]  &177  \\ %\hline
%   theoretical memory bandwidth [GB/s]      &  177 \\ \hline
%          Device to Device [GB/s] & 148.39 \\ \hline
%          Device to Host [GB/s] & 4.46 \\ \hline
%          Host to Host [GB/s]     & 9.44   \\ \hline
%          Host to Device [GB/s] & 3.92 \\ \hline
% %  test memory bandwidth [GB/s]      &  148.4 \\ \hline
%    \end{tabular}
%}
%{\footnotesize The last four rows is tested by  bandwidthtest  of  CUDA 4.1 SDK .}
%\end{table}

%\begin{table}[H] %[htbp]
%  \centering
%  \small
%  \caption{ Memory Bandwidth reported by  bandwidthtest  of  CUDA 4.1 SDK }\label{memorybandwidth}
%  \begin{tabular}{l r} \hline
%          Host to Host      & 9.4411GB/s   \\ \hline
%          Host to Device& 3.9251GB/s \\ \hline
%           Device to Host & 4.4631GB/s \\ \hline
%           Device to Device & 148.3966GB/s \\ \hline
%  \end{tabular}
%  \small
%\end{table}
\subsection{$\vec {r} =\vec{f} - \mathbf{A}\vec {u}$  }

\begin{table}[H]
\centering\caption{ Double precision  GFLOPS  for $\vec {r} =\vec{f} - \mathbf{A}\vec {u}$ in 2D }\label{table_GFLOPs_2D}
\begin{tabular}{|c|c|c|c|c|c|c|}\hline
 &\multicolumn{2}{|c|}{CPU}&\multicolumn{2}{|c|}{GPU} &\multirow{2}{*}{Speedup} \\ \cline{2-5}
 \raisebox{1.5ex}[0pt]{L}&time & Gflops &time &Gflops &  \\\hline
    6      &1.0468e-5   &2.42         &4.5308e-6        &5.60          &2.31 \\ \hline
    7      &3.8158e-5   &2.62         &7.4177e-6        &13.46         &5.14\\ \hline
    8      &1.5440e-4   &2.57         &1.6148e-5        &24.54         &9.56 \\ \hline
    9      &1.7865e-3   &0.88         &4.9640e-5        &31.81         &35.99 \\ \hline
    10     &7.8907e-3   &0.80         &1.8124e-4        &34.78         &43.54 \\ \hline
    11     &3.2138e-2   &0.78         &7.0802e-4        &35.58         &45.39  \\ \hline
    12     &1.3021e-1   &0.80         &2.8167e-3        &35.75         &46.23 \\ \hline
\end{tabular}
\end{table}
%please
%%”……œ±Ìø…÷™
%%
%% 1. µ± $L \leq 8$  ±, CPU ∑Â÷µ double precision GFLOPS $> 2.4$  ≥¨π˝ CPU µƒ¿Ì¬€∑Â÷µ(3.6 GHz float precision),
%%∆‰÷˜“™‘≠“Ú «πÊƒ£Ωœ–° ±cpu cache  √¸÷–¬ Ωœ∏ﬂ, ¥”∂¯ªÒµ√¡ÀΩœ∫√µƒ∑Â÷µ–‘ƒ‹.
%%
%%2.  ÀÊ◊≈πÊƒ£ $L$ ‘ˆ¥Û, º”ÀŸ±»µ•µ˜‘ˆº”.

\begin{figure}[H]
  % Requires \usepackage{graphicx}
\begin{center}
  \includegraphics[width=0.8\textwidth]{fig/2d_residual}
  \caption{Residual for 2D GMG}\label{figure_Residual_2D_GMG}
\end{center}
\end{figure}

\begin{table}[H]
\centering\caption{Kernel time rate for  2D $T_{Vcycle}/ T_{Residual}$ } \label{table_vcycle_res_2D}
    \begin{tabular}{|c|c|c|c|c|c|} \hline
    $L$     & $GMG(1,1)$     &$GMG(1,2)$     &$GMG(2,2)$     &$GMG(2,3)$     &$GMG(3,3)$        \\ \hline
    8           &30            &37            &42              &49            &56      \\ \hline
    9           &18            &22             &26             &30            &34     \\ \hline
    10          &15            &18             &22             &25            &29      \\ \hline
    11          &14            &17             &20             &24            &27   \\ \hline
    12          &13            &17             &20             &23            &27     \\ \hline
    \end{tabular}
\end{table}

\begin{table}[H]
\centering\caption{  Double precision  GFLOPS  for $\vec {r} =\vec{f} - \mathbf{A}\vec {u}$ in 3D}\label{table_GFLOPs_3D}
\begin{tabular}{|c|c|c|c|c|c|c|}\hline
 &\multicolumn{2}{|c|}{CPU}&\multicolumn{2}{|c|}{GPU} &\multirow{2}{*}{Speedup} \\ \cline{2-5}
 \raisebox{1.5ex}[0pt]{L}&time & Gflops &time &Gflops &  \\\hline
    5     &1.2181e-04   &2.36         &2.4494e-05        &11.79         &4.97   \\ \hline
    6     &1.0592e-03   &2.07         &8.9253e-05        &24.58         &11.87  \\ \hline
    7     &9.6409e-03   &1.78         &5.2051e-04        &32.99         &18.52   \\ \hline
    8     &1.3772e-01   &0.99         &5.1200e-03        &26.53         &26.90  \\ \hline
\end{tabular}
\end{table}

\begin{figure}[H]
  % Requires \usepackage{graphicx}
\begin{center}
  \includegraphics[width=0.8\textwidth]{fig/3d_residual}
  \caption{Residual for 3D GMG}\label{figure_Residual_3D_GMG}
\end{center}
\end{figure}

\begin{table}[H]
\centering\caption{Kernel time rate for  3D $T_{Vcycle}/ T_{Residual}$ } \label{table_vcycle_res_3D}
    \begin{tabular}{|c|c|c|c|c|c|} \hline
    $L$     & $GMG(1,1)$     &$GMG(1,2)$     &$GMG(2,2)$     &$GMG(2,3)$ &$GMG(3,3)$        \\ \hline
   5        &25             &33             &39             &46           &53\\ \hline
   6        &21             &27             &33             &38           &44\\ \hline
   7        &14             &18             &22             &25           &29\\ \hline
   8        &10             &13             &16             &18           &21\\ \hline
    \end{tabular}
\end{table}

\subsection{Numerical experiments in 2D}
\begin{example} \label{example2D}
Consider for the model problem \ref{equ1-1-1}, Let
$$\Omega =(0,1)^2 \subset \mathbb{R}^2,$$
$$f(x,y)= \sin(\pi x)\sin(\pi y), \quad (x,y) \in \Omega,$$
$$ tols = 1.0\times 10^{-6}, \mu_f = \mu_b = 1. $$

\end{example}

\begin{table}[H]
        \centering\caption{Iteration numbers and $||\cdot||$ for GPU and CPU }\label{table_error_order2D}
        \begin{tabular}{|l|c|c|c|c|c|c|}\hline
         & \multicolumn{3}{|c|}{$\mbox{CPU}$} & \multicolumn{3}{|c|} { $\mbox{GPU}$}
        \\ \cline{2-7}
        \raisebox{1.5ex}[0pt]{Size} &\#It &$\|\vec{u}-\vec{u}_h\| $  &$\frac{\|\vec{u}-\vec{u}_h\|}{ \|\vec{u}-\vec{u}_{\frac{h}{2}}\|}$ & Its &$\|\vec{u}-\vec{u}_h\| $ &$\frac{\|\vec{u}-\vec{u}_h\|}{ \|\vec{u}-\vec{u}_{\frac{h}{2}}\|}$  \\\hline
        $(2^8+1)^2$     &11  &6.250e-6   &-     &11   &6.250e-6  &-       \\ \hline

        $(2^9+1)^2$     &11  &1.565e-6   &3.99  &11   &1.565e-6  &3.99    \\ \hline

        $(2^{10}+1)^2$  &11  &3.910e-7   &4.00  &11   &3.910e-7  &4.00    \\ \hline

        $(2^{11}+1)^2$  &11  &9.719e-8   &4.02  &11   &9.719e-8  &4.02    \\ \hline

        $(2^{12}+1)^2$  &11  &2.370e-8   &4.10  &11   &2.370e-8  &4.10    \\ \hline
       \end{tabular}
       \end{table}

       \textbf{Conclusion}:Table \ref{table_error_order2D} show that both the GPU programmer and the CPU programmer have saturation of error order in case of 2D.
       Further more,  the GPU programmer and the CPU programmer have the same error order and iteration numbers,
       namely the GPU parallel algorithm reconstructed the CPU serial algorithm.

\begin{table}[H]
\centering\caption{ $\mbox{GPUGMG}$ Solving Time for 2D (Seconds) }\label{table_time_2D}
    \begin{tabular}{|c|c|c|c|c|c|} \hline
    $L_{\theta}$    &$(2^8+1)^2$   &$(2^9+1)^2$ &$(2^{10}+1)^2$  &$(2^{11}+1)^2$    & $(2^{12}+1)^2$  \\ \hline
    0  &1.690e-2  &1.353e-1    &5.270e-1  &2.180e+0      & 9.181e+0       \\ \hline
    1  &7.089e-3  &2.390e-2    &1.067e-1  &4.885e-1      & 2.308e+0       \\ \hline
    2  &4.556e-3  &1.294e-2    &4.594e-2  &2.024e-1      & 8.493e-1       \\ \hline
    3  &4.336e-3  &1.072e-2    &3.494e-2  &1.415e-1      & 5.666e-1       \\ \hline
    4  &4.621e-3  &1.049e-2    &3.276e-2  &1.304e-1      & 5.042e-1       \\ \hline
    5  &5.033e-3  &1.077e-2    &3.252e-2  &1.281e-1      & 4.917e-1        \\ \hline
    6  &5.639e-3  &1.112e-2    &3.287e-2  &1.282e-1      & 4.900e-1        \\ \hline
    7  &6.142e-3  &1.159e-2    &3.324e-2  &1.282e-1      & 4.910e-1        \\ \hline
    8  &6.303e-3  &1.204e-2    &3.375e-2  &1.285e-1      & 4.915e-1        \\ \hline
    9  & -        &1.153e-2    &3.412e-2  &1.291e-1      & 4.906e-1        \\ \hline
    10 & -        &  -         &3.356e-2  &1.299e-1      & 4.924e-1        \\ \hline
    11 & -        &  -         & -        &1.291e-1      & 4.916e-1       \\ \hline
    12 & -        &  -         & -        &  -           & 4.916e-1        \\ \hline
    \end{tabular}
\end{table}

\begin{table}[H]
\centering\caption{ $\mbox{GPUGMG}$  Speed Up  for 2D  }\label{table_speedup_2D}
    \begin{tabular}{|c|c|c|c|c|c|} \hline
    $L_{\theta}$    &$(2^8+1)^2$   &$(2^9+1)^2$ &$(2^{10}+1)^2$  &$(2^{11}+1)^2$    & $(2^{12}+1)^2$  \\ \hline
    0  & 1.00       &1.00          &1.00        &1.00            &1.00      \\ \hline
    1  & 2.38       &5.57          &4.93        &4.46            &3.94      \\ \hline
    2  & 3.71       &10.53         &15.1        &15.37           &16.01     \\ \hline
    3  & 3.91       &13.01          &12.74       &15.01           &14.78    \\ \hline
    4  & 3.63       &13.29          &16.11       &16.66           &18.02      \\ \hline
    5  & 3.36       &13.02          &16.22       &17.00           &18.50     \\ \hline
    6  & 3.00       &12.48          &16.07       &16.98           &18.56     \\ \hline
    7  & 2.76       &11.6          &15.86       &16.99           &18.52      \\ \hline
    8  & 2.85       &11.39          &15.6       &17.02           &18.57       \\ \hline
    9  & -          &12.1          &15.48       &16.86           &18.54      \\ \hline
    10  & -         &-             &15.73       &16.83           &18.49      \\ \hline
    11  & -         &  -           & -          &16.91           &18.45        \\ \hline
    12  & -         &  -           & -          &-               &18.49     \\ \hline
    \end{tabular}
\end{table}

\begin{figure}[H]
  % Requires \usepackage{graphicx}
\begin{center}
  \includegraphics[width=0.8\textwidth]{fig/2d_speedup_nvcc}
  \caption{Speed Up for 2D GMG}\label{figure_Speedup_2D_GMG}
\end{center}
\end{figure}

\textbf{conclusion}:if we take the best case, i.e.,
 17.61 times speed up from table \ref{table_speedup_2D}, it indicate our GPU parallel algorithm and code of GMG has  high
 speedup in case of  2D.

\textbf{conclusion}: From Table \ref{table_speedup_2D} and Figure \ref{figure_Speedup_2D_GMG} we can know:
%%
%%1. ≤ªÕ¨µƒ $L_{\theta}$ æﬂ”–≤ªÕ¨µƒº”ÀŸ±».
%%
%%2. µ±πÊƒ£ $L$ Ωœ¥Û ±£¨º”ÀŸ±»ÀÊ◊≈ $L_{\theta}$ º”¥Û∂¯±‰¥Û(»Á $L=11,12$)
%%
%%3. µ±πÊƒ£ $L$ Ωœ–° ±£¨‘⁄ø™ ºΩ◊∂Œº”ÀŸ±»ÀÊ  $L_{\theta}$ º”¥Û∂¯±‰¥Û£¨÷Æ∫Ûº”ÀŸ±»ÀÊπÊƒ£‘ˆ¥Û∂¯ºı…Ÿ(»Á $L=7,8,9$).
%%
%%   ÷ÆÀ˘“‘º”ÀŸ±»≥ œ÷’‚÷÷∑÷≤º£¨ «”…”⁄µ±À˘–Ë«ÛΩ‚Œ Ã‚πÊƒ£Ωœ–° ±£¨ƒ⁄¥Ê∑√Œ —” ± ”Î GPU»ŒŒÒ¡ø≤ªπª±•µº÷¬≤ø∑÷GPU coresœ–÷√£¨
%%    πµ√ GPU µƒ‘ÀÀ„–‘ƒ‹µ√≤ªµΩ≥‰∑÷∑¢ª”£¨∆‰‘ÀÀ„ÀŸ∂»∑¥∂¯ª·±» CPU ¬˝. ¥”∂¯£¨Œ“√«–Ë“™∫œ¿Ìµƒ—°‘Ò $L_{\theta}$
%%    ≥‰∑÷∑¢ª”CPU”ÎGPUµƒ–≠Õ¨º∆À„ƒ‹¡¶£¨Ã·∏ﬂ“Ïππº∆À„µƒ’˚ÃÂº∆À„–‘ƒ‹.
%%    ‘⁄∆Ωæ˘“‚“Â…œ¿¥Àµ, ’Î∂‘2D«È–ŒŒ“√«»° $L_{\theta}=4 ~or~ 5$ ø… πÀ„∑®¥ÔµΩ◊Ó”≈º”ÀŸ±».

\begin{table}[H]
\centering\caption{ $\mbox{GPUGMG}$ double precision  GFLOPS  for 2D   }\label{table_GFLOPs_2D}
    \begin{tabular}{|c|c|c|c|c|c|} \hline
    $L_{\theta}$    &$(2^8+1)^2$   &$(2^9+1)^2$ &$(2^{10}+1)^2$  &$(2^{11}+1)^2$    & $(2^{12}+1)^2$  \\ \hline
    0     &1.73   &0.8   &0.81   &0.78  &0.74  \\ \hline
    1     &3.88   &4.38  &3.81   &3.36  &2.81  \\ \hline
    2     &6.44   &8.60  &9.30   &8.71  &8.12  \\ \hline
    3     &6.84   &10.67 &12.58  &13.13 &12.81  \\ \hline
    4     &6.33   &10.95 &13.54  &14.45 &14.68  \\ \hline
    5     &5.72   &10.61 &13.65  &14.75 &15.11  \\ \hline
    6     &5.00   &10.17 &13.49  &14.78 &15.19  \\ \hline
    7     &4.53   &9.75  &13.32  &14.74 &15.2  \\ \hline
    8     &4.63   &9.33  &13.11  &14.68 &15.19  \\ \hline
    9     &-      &9.85   &12.93 &14.63  &15.18 \\ \hline
    10    &-      &-      &13.2  &14.57  &15.16  \\ \hline
    11    &-      &-      &-     &14.65  &15.14 \\ \hline
    12    &-      &-      &-     &-      &15.17  \\ \hline
    \end{tabular}
\end{table}

\begin{figure}[H]
  % Requires \usepackage{graphicx}
\begin{center}
  \includegraphics[width=0.8\textwidth]{fig/2d_gflops_nvcc}
  \caption{Gflops for 2D GMG}\label{figure_Gflops_2D_GMG}
\end{center}
\end{figure}

\textbf{conclusion}: If we take the best case, i.e., 14.87 double precision  GFLOPS  at Table\ref{table_GFLOPs_2D} , it makes 8.4\% of  peak performance in case of 2D.

\begin{table}[H]
\centering\caption{ $\mbox{GPUGMG}$  GB/s  for 2D   }\label{table_GBs_2D}
    \begin{tabular}{|c|c|c|c|c|c|} \hline
    $L_{\theta}$    &$(2^8+1)^2$   &$(2^9+1)^2$ &$(2^{10}+1)^2$  &$(2^{11}+1)^2$    & $(2^{12}+1)^2$  \\ \hline
    0  &14.56       &8.56          &6.72        &6.32         &6.24    \\ \hline
    1  &25.28       &33.44         &29.6        &26.64        &22.80    \\ \hline
    2  &44.64       &64.24         &72.08       &67.92        &60.16      \\ \hline
    3  &47.04       &78.96         &96.72       &102.24       &97.12     \\ \hline
    4  &44.16       &81.84         &104.24       &112.64      &115.2       \\ \hline
    5  &40.32       &79.36         &105.04       &114.96      &118.16    \\ \hline
    6  &35.36       &75.76         &104.16       &115.28      &118.88      \\ \hline
    7  &32.16       &72.96         &102.8       &115.04       &118.88     \\ \hline
    8  &34.4        &69.84         &101.36       &114.64      &118.96     \\ \hline
    9  &-           &77.28         &99.92       &114.08       &118.72      \\ \hline
    10 & -          &  -           &103.28       &113.68      &118.56      \\ \hline
    11 & -          &  -           & -           &114.72      &118.48      \\ \hline
    12 & -          &  -           & -           &  -         &118.72       \\ \hline
    \end{tabular}
\end{table}
\textbf{conclusion}: The theoretical peak of  Nvidia Geforce Gtx 480  is 177GB/s ,but its actual measurement is 148.3 GB/s reported by the bandwidthtest utility program from the CUDA 4.1 SDK at our computer. The  actual measurement memory bandwidth peak performance of Host memory is 4.5GB/s.
If we take the best case, i.e., 118.96GB/s at Table\ref{table_GBs_2D} , it makes 80.2\% of the  actual measurement memory bandwidth peak performance in case of 2D.

\begin{table}[H]
\centering\caption{ $\mbox{GPUGMG}$ Memory size  for 2D GMG }\label{table_mem_2D}
    \begin{tabular}{|l|r|r|r|r|r|} \hline
       $L$ &$(2^8+1)^2$   &$(2^9+1)^2$ &$(2^{10}+1)^2$  &$(2^{11}+1)^2$    & $(2^{12}+1)^2$  \\ \hline
    Ndof            & 66049        & 263169     & 1050625        &4198401           &16785409       \\ \hline
    Memory Size     & 242865       & 966323     & 3855029        &15399607          & 61557433        \\ \hline
    Memory Size per dof            & 3.6770       & 3.6719     & 3.6693        &3.6680           &3.6673       \\ \hline
    \end{tabular}
\end{table}

 \textbf{conclusion}: Table \ref{table_mem_2D} shows that the memory space complexity of Algorithm \ref{GMGSolve_GPU} is $O(n)$ in case of 2D.

\subsection{Numerical experiments in 3D}
\begin{example} \label{example3D}
Consider for the model problem \ref{equ1-1-1}, Let
$$\Omega =(0,1)^3 \subset \mathbb{R}^3,$$
$$ f(x,y,z)= \sin(\pi x)\sin(\pi y)\sin(\pi z), \quad (x,y,z) \in \Omega,$$
$$ tols = 1.0\times 10^{-6}, \mu_f = \mu_b = 1. $$
\end{example}

\begin{table}[H]
        \centering\caption{GMG Iteration numbers and $||\cdot||$ for GPU and CPU }\label{table_error_order3D}
        \begin{tabular}{|l|c|c|c|c|c|c|}\hline
         & \multicolumn{3}{|c|}{$\mbox{CPU}$} & \multicolumn{3}{|c|} { $\mbox{GPU}$}
        \\ \cline{2-7}
        \raisebox{1.5ex}[0pt]{Size} &\#It &$\|u-u_h\| $  &$\frac{\|u-u_h\|}{ \|u-u_{\frac{h}{2}}\|}$ & \#It &$\|u-u_h\| $ &$\frac{\|u-u_h\|}{ \|u-u_{\frac{h}{2}}\|}$  \\\hline

        $(2^5+1)^3$   &15  &2.713e-4   &-     &15   &2.713e-4  &-    \\ \hline

        $(2^6+1)^3$   &15  &6.936e-5   &3.91  &15  &6.936e-5   &3.91    \\ \hline

        $(2^{7}+1)^3$ &15  &1.753e-5   &3.97  &15  &1.753e-5   &3.97    \\ \hline

        $(2^{8}+1)^3$ &15  &4.404e-6   &3.98  &15  &4.404e-6   &3.98    \\ \hline

       \end{tabular}
       \end{table}
    \textbf{Conclusion}:Table \ref{table_error_order3D} show that both the GPU programmer and the CPU programmer
     have saturation of error order in case of 3D. Further more,  the GPU programmer and the CPU programmer have the same error order and iteration numbers ,
     namely the GPU parallel algorithm reconstructed the CPU serial algorithm in case of 3D.

%\begin{table}[H]
%        \centering\caption{FMG Iteration numbers and $||\cdot||$ for GPU and CPU }\label{table_error_order3D_fmg}
%        \begin{tabular}{|l|c|c|c|c|c|c|}\hline
%         & \multicolumn{3}{|c|}{$\mbox{CPU}$} & \multicolumn{3}{|c|} { $\mbox{GPU}$}
%        \\ \cline{2-7}
%        \raisebox{1.5ex}[0pt]{Size} &\#It &$\|u-u_h\| $  &$\frac{\|u-u_h\|}{ \|u-u_{\frac{h}{2}}\|}$ & \#It &$\|u-u_h\| $ &$\frac{\|u-u_h\|}{ \|u-u_{\frac{h}{2}}\|}$  \\\hline
%
%        $(2^5+1)^3$   &1  &1.966e-4   &-     &1   &1.966e-4  &-    \\ \hline
%
%        $(2^6+1)^3$   &1  &5.550e-5   &3.54  &1  &5.550e-5   &3.54    \\ \hline
%
%        $(2^{7}+1)^3$ &1  &1.461e-5   &3.79  &1  &1.461e-5   &3.79    \\ \hline
%
%        $(2^{8}+1)^3$ &1  &3.733e-6   &3.91  &1  &3.733e-6   &3.91    \\ \hline
%
%       \end{tabular}
%       \end{table}
%    \textbf{Conclusion}:1. Table \ref{table_error_order3D_fmg} show that both the GPU programmer and the CPU programmer have saturation of error order in case of 3D. Further more,  the GPU programmer and the CPU programmer have the same error order and iteration numbers , namely the GPU parallel algorithm reconstructed the CPU serial algorithm in case of 3D.
%    2. From Table \ref{table_error_order3D_fmg} and Table \ref{table_error_order3D} we can know that for  $\|u-u_h\| $ of one cycle of the FMG is more accurate than the corresponding GMG which with $ tols = 1.0\times 10^{-6}$

\begin{table}[H]
\centering\caption{ $\mbox{GPUGMG}$ New Solving Time for 3D (Seconds) }\label{table_time_3D}
    \begin{tabular}{|c|c|c|c|c|} \hline
    $L_{\theta}$    &$(2^5+1)^3$   &$(2^6+1)^3$ &$(2^{7}+1)^3$  &$(2^{8}+1)^3$    \\ \hline
    0   &1.3560e-2  &1.2955e-1  &1.2623e+0  &1.2564e+1   \\ \hline
    1   &7.0800e-3  &3.0631e-2  &2.0853e-1  &1.8925e+0    \\ \hline
    2   &7.1960e-3  &2.3261e-2  &1.0977e-1  &8.9100e-1      \\ \hline
    3   &8.0207e-3  &2.3354e-2  &1.0240e-1  &7.9275e-1     \\ \hline
    4   &9.0017e-3  &2.4136e-2  &1.0242e-1  &7.8395e-1     \\ \hline
    5   &8.7531e-3  &2.5215e-2  &1.0334e-1  &7.8574e-1     \\ \hline
    6   &-          &2.4936e-2  &1.0444e-1  &7.8652e-1     \\ \hline
    7   &-          &-          &1.0408e-1  &7.8594e-1     \\ \hline
    8   &-          &-          &-          &7.8538e-1     \\ \hline
    \end{tabular}
\end{table}

\begin{table}[H]
\centering\caption{ $\mbox{GPUGMG}$ Speed Up for 3D  }\label{table_speedup_3D}
    \begin{tabular}{|c|c|c|c|c|} \hline
    $L_{\theta}$    &$(2^5+1)^3$   &$(2^6+1)^3$ &$(2^{7}+1)^3$  &$(2^{8}+1)^3$ \\ \hline
    0   &1.00   &1.00   &1.00   &1.00 \\ \hline
    1   &1.91   &4.24   &6.01   &6.63  \\ \hline
    2   &1.87   &5.59   &11.34  &14.13  \\ \hline
    3   &1.67   &5.56   &12.28  &15.84  \\ \hline
    4   &1.49   &5.37   &12.15  &16.01  \\ \hline
    5   &1.53   &5.16   &11.99  &15.97  \\ \hline
    6   &-      &5.2    &11.84  &15.96  \\ \hline
    7   &-      &-      &12.03  &15.98  \\ \hline
    8   &-      &-      &-      &15.99   \\ \hline
    \end{tabular}
\end{table}

\textbf{conclusion}:if we take the best case, i.e.,
 15.40 times speed up from table \ref{table_speedup_3D}, it indicate that our GPU parallel algorithm and code of GMG has  high
 speedup in case of  3D.

\begin{figure}[H]
  % Requires \usepackage{graphicx}
\begin{center}
  \includegraphics[width=0.8\textwidth]{fig/3d_speedup_nvcc}
  \caption{Speed Up for 3D GMG}\label{figure_Speedup_3D_GMG}
\end{center}
\end{figure}

\textbf{conclusion}: From Table \ref{table_speedup_3D} and Figure \ref{figure_Speedup_3D_GMG} we can know:
%% $L_{\theta}$ ∂‘º”ÀŸ±»µƒ”∞œÏ”Î 2D «È–Œœ‡Ω¸. ¿‡À∆µÿ£¨’Î∂‘ 3D «È–ŒŒ“√«»° $L_{\theta} = 3$ algorithm \ref{GMGSolve_GPU} ƒ‹¥ÔµΩ◊Ó∫√µƒº”ÀŸ–‘ƒ‹.

\begin{table}[H]
\centering\caption{ $\mbox{GPUGMG}$ double precision  GFLOPS  for 3D   }\label{table_GFLOPs_3D}
    \begin{tabular}{|c|c|c|c|c|} \hline
    $L_{\theta}$    &$(2^5+1)^3$   &$(2^6+1)^3$ &$(2^{7}+1)^3$  &$(2^{8}+1)^3$    \\ \hline
    0   &1.5    &1.25    &1.01    &0.81    \\ \hline
    1   &2.66   &5.00    &5.89    &5.28    \\ \hline
    2   &2.61   &6.73    &11.56   &11.81   \\ \hline
    3   &2.33   &6.69    &12.47   &13.45   \\ \hline
    4   &2.06   &6.45    &12.45   &13.59    \\ \hline
    5   &2.12   &6.18    &12.33   &13.59    \\ \hline
    6   &-      &6.25    &12.21   &13.57    \\ \hline
    7   &-      &-       &12.25   &13.55    \\ \hline
    8   &-      &-       &-       &13.56   \\ \hline
    \end{tabular}
\end{table}

\begin{figure}[H]
  % Requires \usepackage{graphicx}
\begin{center}
  \includegraphics[width=0.8\textwidth]{fig/3d_gflops_nvcc}
  \caption{Gflops for 3D GMG}\label{figure_Gflops_3D_GMG}
\end{center}
\end{figure}

\textbf{conclusion}:If we take the best case, i.e., 13.34 double precision  GFLOPS  at Table\ref{table_GFLOPs_3D} , it makes 7.5\% of  peak performance in case of 3D.

\begin{table}[H]
\centering\caption{ $\mbox{GPUGMG}$ GB/s   GFLOPS  for 3D   }\label{table_GBs_3D}
    \begin{tabular}{|c|c|c|c|c|} \hline
    $L_{\theta}$    &$(2^5+1)^3$   &$(2^6+1)^3$ &$(2^{7}+1)^3$  &$(2^{8}+1)^3$    \\ \hline
    0               &10.96       &9.44          &7.92           &6.64         \\ \hline
    1               &16.08       &38.64         &46.24          &42.24          \\ \hline
    2               &19.12       &51.6          &90.48          &92.72          \\ \hline
    3               &17.12       &51.36         &97.52          &105.68           \\ \hline
    4               &15.28       &49.52         &97.36         &106.72          \\ \hline
    5               &16.64       &47.52         &96.56         &106.72          \\ \hline
    6               & -          &49.04         &95.52         &106.64         \\ \hline
    7               & -          &  -           &96.32         &106.48         \\ \hline
    8               & -          &  -           & -            &106.64         \\ \hline
    \end{tabular}
\end{table}
\textbf{conclusion}: If we take the best case, i.e., 118.16GB/s at Table\ref{table_GBs_3D} , it makes 79.7\% of  the  actual measurement memory bandwidth peak performance in case of 3D.

\begin{table}[H]
\centering\caption{ $\mbox{GPUGMG}$ Memory size  for 3D   }\label{table3Dmem}
    \begin{tabular}{|l|r|r|r|r|r|} \hline
     $L$      &$(2^5+1)^3$   &$(2^6+1)^3$ &$(2^{7}+1)^3$  &$(2^{8}+1)^3$   \\ \hline
    Ndof           &35937          &274625      & 2146689       & 16974593      \\ \hline
    Mem Size           &119399         &907337      & 7072779       & 55849869      \\ \hline
    Mem Size per dof    &3.3225         &3.3039      & 3.2947      & 3.2902      \\ \hline
    \end{tabular}
\end{table}
\textbf{conclusion}: Table \ref{table3Dmem} shows that the memory space complexity  of Algorithm \ref{GMGSolve_GPU} is $O(n)$ in case of 3D.

\subsection{Numerical Experiment for FMG and FFT}\label{subsec:numer_fmg}
\begin{table}[H]
\centering\caption{$\|u-u_h\|_2$ for GPU and CPU }\label{table_fmg_error_2D}
    \begin{tabular}{|l|c|c|c|c|c|}\hline
         & \multicolumn{2}{|c|}{$\mbox{CPU}$} & \multicolumn{2}{|c|} { $\mbox{GPU}$} \\ \cline{2-5}
        \raisebox{1.5ex}[0pt]{Size} &$\|u-u_h\|_2 $  &$\frac{\|u-u_h\|_2}{ \|u-u_{\frac{h}{2}}\|_2}$ &$\|u-u_h\|_2 $ &$\frac{\|u-u_h\|_2}{ \|u-u_{\frac{h}{2}}\|_2}$  \\\hline
        $(2^8+1)^2$       &5.207e-6   &-        &5.207e-6  &-       \\ \hline

        $(2^9+1)^2$       &1.310e-6   &3.97     &1.310e-6  &3.97    \\ \hline

        $(2^{10}+1)^2$    &3.284e-7   &3.99     &3.284e-7  &3.99    \\ \hline

        $(2^{11}+1)^2$    &8.221e-8   &3.99     &8.221e-8  &3.99    \\ \hline

        $(2^{12}+1)^2$    &2.057e-8   &4.00     &2.057e-8  &4.00    \\ \hline
    \end{tabular}
\end{table}

\begin{table}[H]
\centering\caption{ $\mbox{GPUFMG}$ Solving Time for 2D (Seconds)
}\label{table_fmg_time_2d}
    \begin{tabular}{|c|c|c|c|c|c|} \hline
    $L_{\theta}$    &$(2^8+1)^2$   &$(2^9+1)^2$ &$(2^{10}+1)^2$  &$(2^{11}+1)^2$    & $(2^{12}+1)^2$  \\ \hline
    0               &6.640e-3   &3.307e-2       &1.524e-1     &6.460e-1      &2.657e+0       \\ \hline
    1               &5.285e-3   &1.413e-2       &3.818e-2     &1.589e-1      &6.154e-1      \\ \hline
    2               &4.887e-3   &1.119e-2       &2.289e-2     &7.733e-2      &2.891e-1       \\ \hline
    3               &4.884e-3   &1.051e-2       &2.000e-2     &5.622e-2      &2.061e-1       \\ \hline
    4               &4.812e-3   &1.057e-2       &1.941e-2     &5.321e-2      &1.883e-1       \\ \hline
    5               &4.820e-3   &1.053e-2       &1.924e-2     &5.265e-2      &1.858e-1       \\ \hline
    6               &5.006e-3   &1.037e-2       &1.928e-2     &5.247e-2      &1.834e-1       \\ \hline
    7               &5.130e-3   &1.067e-2       &1.938e-2     &5.292e-2      &1.831e-1        \\ \hline
    8               &4.696e-3   &1.057e-2       &1.937e-2     &5.308e-2      &1.833e-1       \\ \hline
    9               & -         &1.002e-2       &1.937e-2     &5.075e-2      &1.849e-1       \\ \hline
    10              & -         &  -            &1.894e-2     &5.236e-2      &1.839e-1       \\ \hline
    11              & -         &  -            & -           &5.240e-2      &1.830e-1       \\ \hline
    12              & -         &  -            & -           &  -           &1.828e-1       \\ \hline
    \end{tabular}
\end{table}

\begin{table}[H]
\centering\caption{ $\mbox{GPUFMG}$ Speed Up  for 2D}\label{table_fmg_speepup_2d}
    \begin{tabular}{|c|c|c|c|c|c|} \hline
    $L_{\theta}$    &$(2^8+1)^2$   &$(2^9+1)^2$ &$(2^{10}+1)^2$  &$(2^{11}+1)^2$    & $(2^{12}+1)^2$  \\ \hline
    0&              1.00            &1.00        &1.00           &1.00               &1.00   \\ \hline
    1&              1.25            &2.31       &4.01            &4.07              &4.3     \\ \hline
    2&              1.37            &2.97       &6.67           &8.37               &9.16    \\ \hline
    3&              1.36            &3.13       &7.67           &11.49              &12.84   \\ \hline
    4&              1.40            &3.14       &7.87           &12.12              &14.06   \\ \hline
    5&              1.38            &3.15       &7.94           &12.3               &14.25   \\ \hline
    6&              1.32            &3.19       &7.92           &12.28              &14.43   \\ \hline
    7&              1.30            &3.10       &7.93           &12.22              &14.45    \\ \hline
    8&              1.43            &3.13       &7.91           &12.19              &14.44    \\ \hline
    9&              -               &3.28       &7.93           &12.72              &14.33    \\ \hline
    10&             -               &-          &8.05           &12.34              &14.41    \\ \hline
    11&             -               &-          &-              &12.33              &14.48    \\ \hline
    12&             -               &-          &-              &-                  &14.49    \\ \hline

    \end{tabular}
\end{table}

\begin{figure}[H]
  % Requires \usepackage{graphicx}
\begin{center}
  \includegraphics[width=0.8\textwidth]{fig/2DFMG_Speedup}
  \caption{Speed Up for 2D FMG}\label{Speedup_2D_FMG}
\end{center}
\end{figure}

\begin{table}[H]
\centering\caption{ $\mbox{GPUFMG}$ Gflops  for 2D   }\label{table_fmg_gflops_2d}
    \begin{tabular}{|c|c|c|c|c|c|} \hline
    $L_{\theta}$    &$(2^8+1)^2$   &$(2^9+1)^2$ &$(2^{10}+1)^2$  &$(2^{11}+1)^2$    & $(2^{12}+1)^2$  \\ \hline
    0&              1.62&           1.16&        0.90&             0.82&            0.8      \\ \hline
    1&              1.31&           2.51&        3.22&             2.86&            2.92     \\ \hline
    2&              1.43&           3.57&        6.41&             6.94&            7.32     \\ \hline
    3&              1.43&           3.92&        7.89&             11.02&           11.83    \\ \hline
    4&              1.45&           3.92&        8.21&             11.96&           13.70     \\ \hline
    5&              1.46&           3.89&        8.33&             12.2&            14.07     \\ \hline
    6&              1.39&           4.02&        8.35&             12.29&           14.20     \\ \hline
    7&              1.35&           3.85&        8.25&             12.17&           14.20     \\ \hline
    8&              1.51&           3.86&        8.26&             12.13&           14.17     \\ \hline
    9&              -&              4.25&        8.32&             12.14&           14.17     \\ \hline
    10&             -&              -&           8.56&             12.27&           14.17     \\ \hline
    11&             -&              -&              -&             12.34&           14.20     \\ \hline
    12&             -&              -&              -&             -&               14.22    \\ \hline

    \end{tabular}
\end{table}

\begin{figure}[H]
  % Requires \usepackage{graphicx}
\begin{center}
  \includegraphics[width=0.8\textwidth]{fig/2DFMG_Gflops}
  \caption{Gflops for 2D FMG}\label{Gflops_2D_FMG}
\end{center}
\end{figure}

\begin{table}[H]
\centering\caption{ $\mbox{GPUFMG}$ GB  for 2D   }\label{table_gb_2d}
    \begin{tabular}{|c|c|c|c|c|c|} \hline
    $L_{\theta}$    &$(2^8+1)^2$   &$(2^9+1)^2$ &$(2^{10}+1)^2$  &$(2^{11}+1)^2$    & $(2^{12}+1)^2$  \\ \hline
    0&              12.96&      9.28&           7.20&        6.56&      6.40       \\ \hline
    1&              10.48&      20.08&          25.76&      22.88&      23.36 \\ \hline
    2&              11.44&      28.56&          51.28&      55.52&      58.56 \\ \hline
    3&              11.44&      31.36&          63.12&      88.16&      94.64 \\ \hline
    4&              11.60&      31.36&          65.68&      95.68&      109.60 \\ \hline
    5&              11.68&      31.12&          66.64&      97.60&      112.56 \\ \hline
    6&              11.12&      32.16&          66.80&      98.32&      113.60 \\ \hline
    7&              10.80&      30.80&          66.00&      97.36&      113.60 \\ \hline
    8&              12.08&      30.88&          66.08&      97.04&      113.36 \\ \hline
    9&              -&          34.00&          66.56&      97.12&      113.36 \\ \hline
    10&             -&          -&              68.48&      98.16&      113.36 \\ \hline
    11&             -&          -&              -&          98.72&      113.60 \\ \hline
    12&             -&          -&              -&          -&          113.76 \\ \hline

    \end{tabular}
\end{table}

\begin{table}[H]
        \centering\caption{ 3D FMG $\|u-u_h\|_2$ for GPU and CPU }\label{table_fmg_error_3d}
        \begin{tabular}{|l|c|c|c|c|}\hline
         & \multicolumn{2}{|c|}{$\mbox{CPU}$} & \multicolumn{2}{|c|} { $\mbox{GPU}$}
        \\ \cline{2-5}
        \raisebox{1.5ex}[0pt]{Size} &$\|u-u_h\|_2 $  &$\frac{\|u-u_h\|_2}{ \|u-u_{\frac{h}{2}}\|_2}$ &$\|u-u_h\|_2 $ &$\frac{\|u-u_h\|_2}{ \|u-u_{\frac{h}{2}}\|_2}$  \\\hline

        $(2^5+1)^3$    & 1.966e-4   &-      &1.966e-4   &-    \\ \hline

        $(2^6+1)^3$    &5.550e-5   &3.54    &5.550e-5   &3.54    \\ \hline

        $(2^{7}+1)^3$  &1.461e-5   &3.92    &1.461e-5   &3.92    \\ \hline

        $(2^{8}+1)^3$  &3.733e-6   &3.91    &3.733e-6   &3.91    \\ \hline

       \end{tabular}
\end{table}

\begin{table}[H]
\centering\caption{ $\mbox{GPUFMG}$ Solving Time for 3D (Seconds)
}\label{table_gmg_time_3d}
    \begin{tabular}{|c|c|c|c|c|} \hline
    $L_{\theta}$    &$(2^5+1)^3$   &$(2^6+1)^3$ &$(2^{7}+1)^3$  &$(2^{8}+1)^3$    \\ \hline
    0               &4.916e-3     &4.270e-2   &3.638e-1      &3.361e+0      \\ \hline
    1               &4.330e-3     &1.496e-2   &6.665e-2      &5.059e-1       \\ \hline
    2               &4.480e-3     &1.325e-2   &4.312e-2      &2.796e-1       \\ \hline
    3               &4.537e-3     &1.334e-2   &3.883e-2      &2.519e-1       \\ \hline
    4               &4.690e-3     &1.333e-2   &4.160e-2      &2.525e-1      \\ \hline
    5               &4.289e-3     &1.334e-2   &4.162e-2      &2.495e-1        \\ \hline
    6               & -            &1.306e-2  &4.156e-2      &2.518e-1       \\ \hline
    7               & -            &  -       &3.902e-2      &2.497e-1      \\ \hline
    8               & -            &  -         & -          &2.482e-1      \\ \hline
    \end{tabular}
\end{table}

\begin{table}[H]
\centering\caption{ $\mbox{GPUFMG}$ Speed Up for 3D  }\label{table_fmg_speedup_3d}
    \begin{tabular}{|c|c|c|c|c|} \hline
    $L_{\theta}$    &$(2^5+1)^3$   &$(2^6+1)^3$ &$(2^{7}+1)^3$  &$(2^{8}+1)^3$ \\ \hline
    0               &1.00           &1.00       &1.00        &1.00             \\ \hline
    1               &1.14           &2.86       &5.46        &6.64              \\ \hline
    2               &1.10           &3.23       &8.43        &12.08             \\ \hline
    3               &1.09           &3.16       &8.70        &13.40             \\ \hline
    4               &1.07           &3.2        &8.72        &13.35             \\ \hline
    5               &1.15           &3.21       &8.76        &13.56             \\ \hline
    6               &-              &3.26       &8.76        &13.38             \\ \hline
    7               &-              &-          &9.27        &13.56             \\ \hline
    8               &-              &-          &-           &13.66             \\ \hline

    \end{tabular}
\end{table}

\begin{figure}[H]
  % Requires \usepackage{graphicx}
\begin{center}
  \includegraphics[width=0.8\textwidth]{fig/3DFMG_Speedup}
  \caption{Speedup for 3D FMG}\label{Speedup_3D_FMG}
\end{center}
\end{figure}

\begin{table}[H]
\centering\caption{ $\mbox{GPUFMG}$ Gflops  for 3D   }\label{table_fmg_gflops_3d}
    \begin{tabular}{|c|c|c|c|c|} \hline
    $L_{\theta}$    &$(2^5+1)^3$   &$(2^6+1)^3$ &$(2^{7}+1)^3$  &$(2^{8}+1)^3$    \\ \hline
    0               &1.34           &1.12       &0.98           &0.82   \\ \hline
    1               &1.01           &3.14       &5.00           &5.07   \\ \hline
    2               &0.97           &3.73       &8.84           &10.65  \\ \hline
    3               &0.96           &3.71       &9.34           &12.20  \\ \hline
    4               &0.92           &3.70       &9.27           &12.31  \\ \hline
    5               &1.03           &3.69       &9.28           &12.31  \\ \hline
    6               &-              &3.82       &9.28           &12.30  \\ \hline
    7               &-              &-          &9.32           &12.30  \\ \hline
    8               &-              &-          &-              &12.32  \\ \hline
    \end{tabular}
\end{table}

\begin{figure}[H]
  % Requires \usepackage{graphicx}
\begin{center}
  \includegraphics[width=0.8\textwidth]{fig/3DFMG_Gflops}
  \caption{Gflops for 3D FMG}\label{Gflops_3D_FMG}
\end{center}
\end{figure}

\begin{table}[H]
\centering\caption{ $\mbox{GPUFMG}$ GB/s  for 3D   }\label{table_fmg_gb_3d}
    \begin{tabular}{|c|c|c|c|c|} \hline
    $L_{\theta}$    &$(2^5+1)^3$   &$(2^6+1)^3$ &$(2^{7}+1)^3$  &$(2^{8}+1)^3$    \\ \hline
    0               &10.72          &8.96       &7.84           &6.56        \\ \hline
    1               &8.08           &25.12      &40.00          &40.56       \\ \hline
    2               &7.76           &29.84      &70.72          &85.20       \\ \hline
    3               &7.68           &29.68      &74.72          &97.60       \\ \hline
    4               &7.36           &29.60      &74.16          &98.48       \\ \hline
    5               &8.24           &29.52      &74.24          &98.48       \\ \hline
    6               &-              &30.56      &74.24          &98.40       \\ \hline
    7               &-              &-          &74.56          &98.40       \\ \hline
    8               &-              &-          &-              &98.56       \\ \hline

    \end{tabular}
\end{table}

%\begin{table}[H]
%\centering\caption{ $\mbox{FFT}$ Solving Time for 2D Poisson (Seconds)}\label{table_time_fft_2d}
%    \begin{tabular}{|c|c|c|} \hline
%    $Ndof$          &ker\_time    &total\_time     \\ \hline
%    $(2^8+1)^2$         &8.244e-4     &3.467e-3        \\ \hline
%    $(2^9+1)^2$         &2.166e-3     &1.133e-2        \\ \hline
%    $(2^{10}+1)^2$        &7.066e-3     &4.004e-2        \\ \hline
%    $(2^{11}+1)^2$        &2.866e-2     &1.565e-1        \\ \hline
%    $(2^{12}+1)^2$        &1.203e-1     &6.261e-1        \\ \hline
%    \end{tabular}
%\end{table}
%
%\begin{table}[H]
%\centering\caption{ $\mbox{FFT}$ Solving Time for 3D Poisson (Seconds)}\label{table_time_fft_3d}
%    \begin{tabular}{|c|c|c|} \hline
%    $Ndof$          &ker\_time    &total\_time    \\ \hline
%    $(2^5+1)^3$         &5.035e-4     &2.042e-3        \\ \hline
%    $(2^6+1)^3$         &2.233e-3     &1.138e-2        \\ \hline
%    $(2^7+1)^3$        &1.528e-2     &7.985e-2       \\ \hline
%    $(2^8+1)^3$        &1.298e-1     &6.426e-1        \\ \hline
%    \end{tabular}
%\end{table}
\subsection{FFT Result}
\begin{table}[H]
\centering\caption{ $\|u-u_h\|_2 $ for 2D}\label{table_error_fft_fmg_2d}
    \begin{tabular}{|c|c|c|c|c|c|c|} \hline
    $L$ &FFT      &FMG(1,1) &FMG(1,2)  &FMG(2,2)    &FMG(2,3)&FMG(3,3)  \\ \hline
   8  &6.226e-6 &3.764e-5  &4.923e-6  &3.978e-6  &2.792e-6  &2.846e-6\\ \hline
   9  &1.563e-6 &1.001e-5  &1.242e-6  &1.004e-6  &7.028e-7  &7.145e-7\\ \hline
   10 &3.914e-7 &2.618e-6  &3.113e-7  &2.518e-7  &1.762e-7  &1.790e-7\\ \hline
   11 &9.797e-8 &6.766e-7  &7.791e-8  &6.304e-8  &4.411e-8  &4.479e-8\\ \hline
   12 &2.450e-8 &1.735e-7  &1.948e-8  &1.577e-8  &1.103e-8  &1.120e-8\\ \hline
%   13 &6.412e-9 &4.421e-8  &4.871e-9  &3.944e-9  &2.759e-9  &2.801e-9\\ \hline
    \end{tabular}
\end{table}

\begin{table}[H]
\centering\caption{ $\mbox{Ker\_time}$ for 2D (s) }\label{table_kertime_fft_gmg_2D}
    \begin{tabular}{|c|c|c|c|c|c|c|} \hline
    $L$    &$FFT$       &FMG(1,1)    &FMG(1,2)      &FMG(2,2)    & FMG(2,3)    &FMG(3,3)  \\ \hline
   8          &5.706e-4    &2.378e-3   &2.776e-3   &3.272e-3  &3.744e-3   &4.194e-3\\ \hline
   9          &1.314e-3    &3.611e-3   &4.260e-3   &4.980e-3  &5.617e-3   &6.348e-3\\ \hline
   10         &4.373e-3    &7.434e-3   &8.770e-3   &1.008e-2  &1.144e-2   &1.282e-2\\ \hline
   11         &1.935e-2    &2.203e-2   &2.571e-2   &2.945e-2  &3.317e-2   &3.701e-2\\ \hline
   12         &8.864e-2    &7.860e-2   &9.167e-2   &1.049e-1  &1.180e-1   &1.310e-1\\ \hline
    \end{tabular}
\end{table}

\begin{table}[H]
\centering\caption{ $\mbox{Ker\_time}$ for 2D (s) }\label{table_kertime_fft_gmg_2D1}
    \begin{tabular}{|c|c|c|c|c|c|c|} \hline
    $L$    &$FFT$       &F(1,1)    &F(1,2)      &F(2,2)    & F(2,3)    &F(3,3)  \\ \hline
   8          &8.019e-4    &2.378e-3   &2.776e-3   &3.272e-3  &3.744e-3   &4.194e-3\\ \hline
   9          &3.739e-3    &3.611e-3   &4.260e-3   &4.980e-3  &5.617e-3   &6.348e-3\\ \hline
   10         &1.102e-2    &7.434e-3   &8.770e-3   &1.008e-2  &1.144e-2   &1.282e-2\\ \hline
   11         &4.077e-2    &2.203e-2   &2.571e-2   &2.945e-2  &3.317e-2   &3.701e-2\\ \hline
   12         &1.364e-1    &7.860e-2   &9.167e-2   &1.049e-1  &1.180e-1   &1.310e-1\\ \hline
    \end{tabular}
\end{table}

\textcolor{red}{For table \ref{table_kertime_fft_gmg_2D} FFT size is $2^L \times 2^L$, table \ref{table_kertime_fft_gmg_2D1} FFT size is $(2^L + 1)^2$.}

\begin{table}[H]
\centering\caption{ $\|u-u_h\|_2 $ for 3D}\label{table_error_fft_fmg_3d}
    \begin{tabular}{|c|c|c|c|c|c|c|} \hline
    $L$ & FFT    &FMG(1,1) &FMG(1,2)  &FMG(2,2)    &FMG(2,3)    &FMG(3,3)  \\ \hline
    5 &2.841e-4 &6.509e-3  &2.733e-3  &1.246e-3  &7.873e-4  &5.296e-4\\ \hline
    6 &7.100e-5  &2.685e-3  &9.469e-4  &3.930e-4  &2.426e-4  &1.608e-4\\ \hline
    7 &1.774e-5 &1.032e-3  &2.988e-4  &1.125e-4  &6.751e-5  &4.394e-5\\ \hline
    8 &4.437e-6 &3.803e-4  &8.880e-5  &3.049e-5  &1.784e-5  &1.145e-5\\ \hline
%    9 & 1.104e-06 &1.364e-4  &2.534e-5  &8.005e-6  &4.592e-6  &2.917e-6\\ \hline
    \end{tabular}
\end{table}

\begin{table}[H]
\centering\caption{ $\mbox{Ker\_time}$ for 3D(s)}\label{table_kertime_fft_gmg_3D}
    \begin{tabular}{|c|c|c|c|c|c|c|} \hline
    $L$    &FFT        &FMG(1,1)     &FMG(1,2)     &FMG(2,2)    &FMG(2,3)    &FMG(3,3)  \\ \hline
   5       &3.459e-4   &1.611e-3   &1.932e-3   &2.382e-3  &2.738e-3  &3.186e-3\\ \hline
   6       &1.507e-3   &3.711e-3   &4.474e-3   &5.335e-3  &6.098e-3  &6.986e-3\\ \hline
   7       &1.171e-2   &1.342e-2   &1.586e-2   &1.846e-2  &2.094e-2  &2.352e-2\\ \hline
   8       &1.055e-1   &8.566e-2   &1.007e-1   &1.155e-1  &1.302e-1  &1.456e-1\\ \hline
    \end{tabular}
\end{table}

\begin{table}[H]
\centering\caption{ $\mbox{Ker\_time}$ for 3D(s)}\label{table_kertime_fft_gmg_3D1}
    \begin{tabular}{|c|c|c|c|c|c|c|} \hline
    $L$    &FFT        &F(1,1)     &F(1,2)     &F(2,2)    &F(2,3)    &F(3,3)  \\ \hline
   5          &5.102e-4   &1.611e-3   &1.932e-3   &2.382e-3  &2.738e-3  &3.186e-3\\ \hline
   6          &1.890e-3   &3.711e-3   &4.474e-3   &5.335e-3  &6.098e-3  &6.986e-3\\ \hline
   7          &5.884e-2   &1.342e-2   &1.586e-2   &1.846e-2  &2.094e-2  &2.352e-2\\ \hline
   8          &1.893e-1   &8.566e-2   &1.007e-1   &1.155e-1  &1.302e-1  &1.456e-1\\ \hline
    \end{tabular}
\end{table}

\textcolor{red}{For table \ref{table_kertime_fft_gmg_3D} FFT size is $2^{3L}$, table \ref{table_kertime_fft_gmg_3D1} FFT size is $(2^L + 1)^3$.}
